# Supplementary material for: The Writing is on the Wall: Analyzing the Boom of Inscriptions and its Impact on Rollup Performance and Cost Efficiency
Source: arXiv:2404.11189 source file (2024-04-17)
Supplement: Supplementary file 1 [file appendix.tex]

\newpage

\section{Extra Figures and Tables}

\begin{figure}[!ht]
  \centering
        \includegraphics[width=0.9\linewidth]{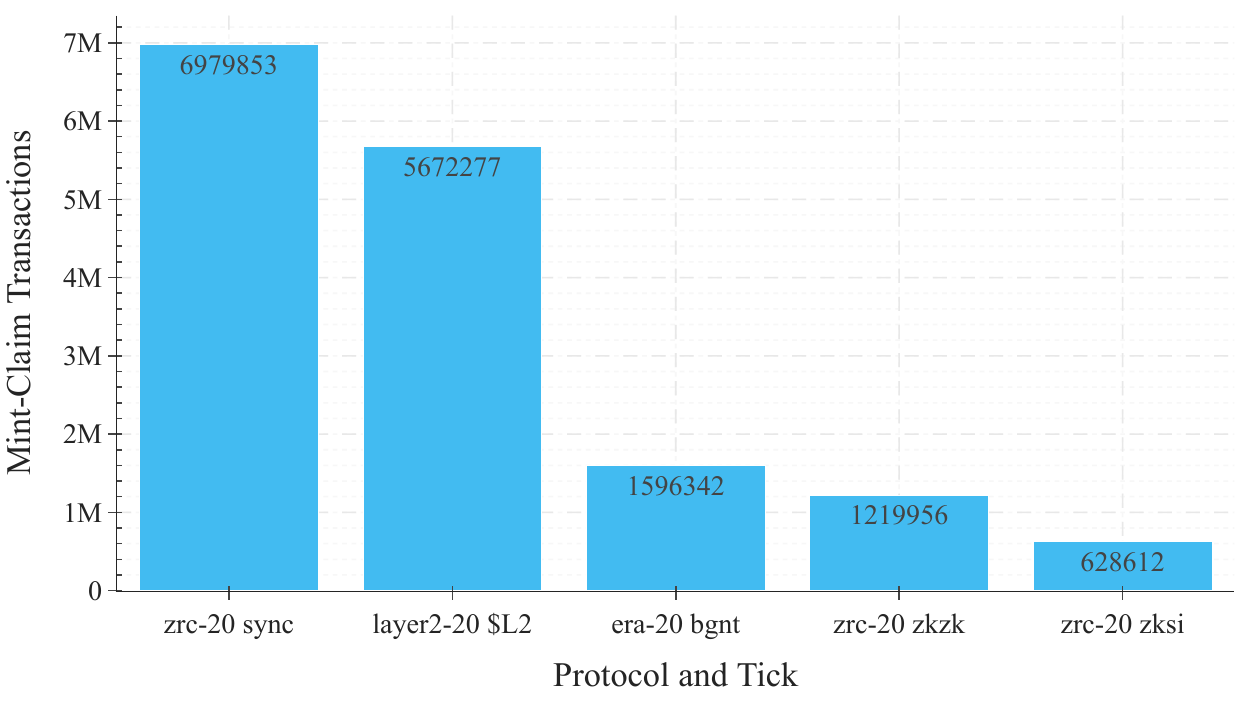} 
    \caption{Top 5 minted protocol-tick on zkSync Era}
    \label{fig:top5mint}
\end{figure}

\begin{figure}[!ht]
  \centering
        \includegraphics[width=0.9\linewidth]{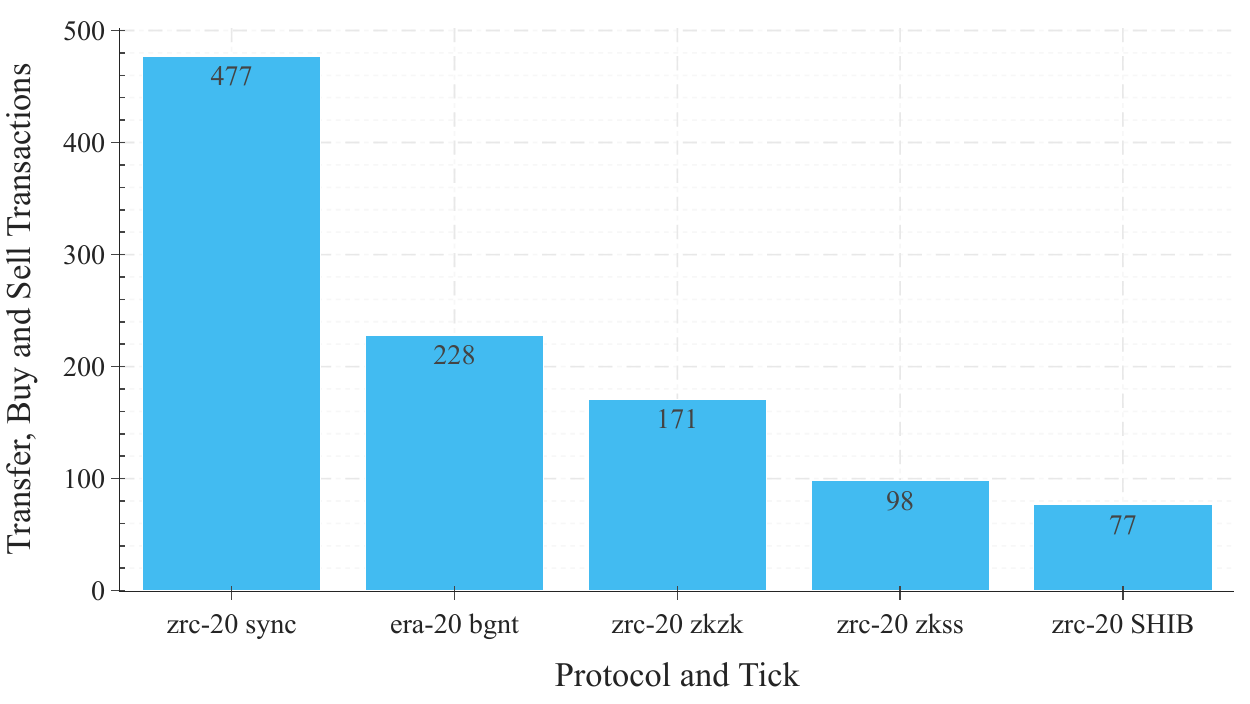} 
    \caption{Top 5 transfered protocol-tick on zkSync Era}
    \label{fig:top5transfer}
\end{figure}

%\begin{figure*}[!ht]
%  \centering
%        \includegraphics[width=0.9\linewidth]{images/buyselltransfer-zksync.png} 
%    \caption{Trading activity (daily buy, sell and transfer transaction) of inscription on zkSync Era}
%    \label{fig:buyselltransfer}
%\end{figure*}
